# Supplementary material for: Time Dependence in Non-Autonomous Neural ODEs
Source: arXiv:2005.01906 source file (2020-05-06)
Supplement: Supplementary file 1 [file appendix.tex]

% %%%%%%%% ICML 2020 EXAMPLE LATEX SUBMISSION FILE %%%%%%%%%%%%%%%%%

% \documentclass{article}

% % Recommended, but optional, packages for figures and better typesetting:
% \usepackage{microtype}
% \usepackage{graphicx}
% \usepackage{subfigure}
% \usepackage{amsfonts}
% \usepackage{makecell}
% \usepackage{paralist}

% \newcommand{\nanode}{NANODE}
% \newcommand{\hypernetwork}{Hypernetwork}
% \newcommand{\basisparams}{\alpha}
% \usepackage{amssymb,amsmath,amsthm}
% \usepackage{tikz}
% \usetikzlibrary{matrix,calc}
% \usepackage{booktabs} % for professional tables
% \usepackage{enumitem}
% % hyperref makes hyperlinks in the resulting PDF.
% % If your build breaks (sometimes temporarily if a hyperlink spans a page)
% % please comment out the following usepackage line and replace
% % \usepackage{icml2020} with \usepackage[nohyperref]{icml2020} above.
% \usepackage{hyperref}

% % Attempt to make hyperref and algorithmic work together better:
% \newcommand{\theHalgorithm}{\arabic{algorithm}}

% % Use the following line for the initial blind version submitted for review:
% \usepackage{icml2020}

% % If accepted, instead use the following line for the camera-ready submission:
% %\usepackage[accepted]{icml2020}

% % The \icmltitle you define below is probably too long as a header.
% % Therefore, a short form for the running title is supplied here:
% \icmltitlerunning{Non-Autonomous Neural ODEs}
 
% \begin{document}

% \twocolumn[
% \icmltitle{Supplementary Materials}

% % It is OKAY to include author information, even for blind
% % submissions: the style file will automatically remove it for you
% % unless you've provided the [accepted] option to the icml2020
% % package.

% % List of affiliations: The first argument should be a (short)
% % identifier you will use later to specify author affiliations
% % Academic affiliations should list Department, University, City, Region, Country
% % Industry affiliations should list Company, City, Region, Country

% % You can specify symbols, otherwise they are numbered in order.
% % Ideally, you should not use this facility. Affiliations will be numbered
% % in order of appearance and this is the preferred way.
% \icmlsetsymbol{equal}{*}

% \begin{icmlauthorlist}
% \icmlauthor{Aeiau Zzzz}{goo}
% \icmlauthor{Bauiu C.~Yyyy}{goo}
% \icmlauthor{Cieua Vvvvv}{goo}
% \end{icmlauthorlist}

% % You may provide any keywords that you
% % find helpful for describing your paper; these are used to populate
% % the "keywords" metadata in the PDF but will not be shown in the document
% \icmlkeywords{Machine Learning, ICML}

% \vskip 0.3in
% ]

% % this must go after the closing bracket ] following \twocolumn[ ...

% % This command actually creates the footnote in the first column
% % listing the affiliations and the copyright notice.
% % The command takes one argument, which is text to display at the start of the footnote.
% % The \icmlEqualContribution command is standard text for equal contribution.
% % Remove it (just {}) if you do not need this facility.

% %\printAffiliationsAndNotice{}  % leave blank if no need to mention equal contribution
% %\printAffiliationsAndNotice{\icmlEqualContribution} % otherwise use the standard text.

% \newpage 

% \appendix
% \section{Appendix}

% \subsection{Experimental Details}

% \subsubsection{Image Classification}

% We conducted our CIFAR10 and CIFAR100 image classification experiments with each model trained on a single GPU, no use of data augmentation, and no pre-training.

% We used architectures of the kind illustrated in Figure 1 of the main text for all experiments. Our residual flow blocks leverage the Bottleneck Residual structure with $1 \times 1 \times 64$, $3 \times 3 \times 64$, and $1 \times 1 \times 256$ CNN layers.

% \begin{table}[h]
% \label{table:cifar_performance_stats}
% \caption{Distribution statistics for comparison of various architectures for CIFAR-10 and CIFAR-100 image classification tasks.}
% \begin{center}
% \begin{small}
% \begin{sc}
% \resizebox{.95\columnwidth}{!}{%
% \begin{tabular}{lcccr}
% \toprule
% \makecell{MODEL} & \makecell{CIFAR10 \\ Acc (\%)} & \makecell{CIFAR10 \\ STDDEV} & \makecell{CIFAR100 \\ Acc (\%)} & \makecell{CIFAR100 \\ STDDEV} \\
% \midrule
% \makecell{Auto} & 82.98 & 1.1 & 50.33 &  0.3 \\
% \makecell{AppNODE} & 83.20 & 1.3 & 60.68 &  1.7 \\
% \makecell{Con. ResNet} & 82.35 & 2.2 & 54.69 & 0.8  \\
% \makecell{ Uncon. ResNet} & 86.72 & 1.6 & 60.91 & 2.4  \\
% \makecell{B-{\nanode}-10} & 84.38 & 1.24 & 51.66 & 2.0   \\
% \makecell{T-{\nanode}-10} & 90.10 & 1.9 & 66.49 &  1.2  \\
% \makecell{B-{\nanode}-100} & 93.22 & 0.5 & 64.06 & 1.2   \\
% \bottomrule
% \end{tabular}%
% }
% \end{sc}
% \end{small}
% \end{center}
% \end{table}




% \subsubsection{Video Prediction}

% We used 2 conditioning frames to predict 10 future ahead in both Moving MNIST and BAIR Robot Pushing experiments. We used no pretraining or data augmentation. Training for each model was conducted on a single GPU.

% For Moving MNIST, we log losses after 10 hours of training. For BAIR Robot Pushing Small, we log losses after 40 hours of training. 

% \subsubsection{A.1 Hypernetworks Experiments}

% Here we discuss the {\hypernetwork}s results in more depth. For the direct {\hypernetwork} framing, specified in the main text and again in Eqn. \ref{eq:hyper_direct_appendix} (below), we were unable to observe any stable training for what we surmise are the same conditioning reasons discussed in Section 2.4 of the main text. 
% We swept multiple $\Psi$ configurations, varying the activations, depths, and widths of the network. 

% For the gating variant specified in the main text and again in Eqn \ref{eq:hyper_gate_appendix} (below), we instantiated a separate Dense {\hypernetwork} with 4 layers of width 512. This dense network was trained to take in scalar time $t$ and output a sigmoid vector equating to the weighting to use when combining dynamics. We observed that this system resolved conditioning challenges and did not collapse as readily as the direct variant. However, for $dt=0.05$ and $t_{0} = 0, t_{1} = 1$, increased dynamics did not improve performance, but actually lowered it. For $dt=0.01$, as we increased both the effective depth of the network and the precision of the adjoint method performing gradient updates, we began to observe improvements on the training set but not the test set, suggesting this hypernetwork approach is more susceptible to over-fitting than trigonometric polynomial variants. Experimenting with SDE ideas and regularizing schemes in this context is a direction for future work. 


% \begin{figure}[!th]
%         \includegraphics[width=\linewidth]{Figures/hypernetworks.pdf}
%         \caption{Results for gating {\hypernetwork}s  with $dt = 0.05$. We were able to train Gating {\hypernetwork}s but observed diminishing performance (particularly for CIFAR100) as we increased the number of gates. Ultimately, gate\_dim (or embedding\_dim) of $1$, an autonomous network, performed best.}
%         \label{fig:hyper_unstable}
% \end{figure}

% \begin{equation}\label{eq:hyper_direct_appendix}
% W_{t,ij} = \Psi([\vec{v_{ij}}, t]) 
% \end{equation}

% \textbf{Direct {\hypernetwork} framing}:
% In Eqn. \ref{eq:hyper_direct_appendix}, we state the definition of the hypernetwork variant that directly computes weights $W_{t,ij}$. Above, $\vec{v_{ij}}$, which represents a learned scalar or a vector state embedding for a given weight $W_{t,ij}$, is augmented with $t$ and passed to Neural Network $\Psi$.

% \textbf{Gating {\hypernetwork} framing}:
% In the gating variant, by contrast, we could learn a $\sigma{(t)}$ gating mechanism that combines $d$ different potential hidden dynamics $f$, each initialized via a standard initialization scheme, in a proportion defined by a sigmoid. This results in 
% \begin{equation} \label{eq:hyper_gate_appendix}
% \frac{d\textbf{h}_{t}}{dt} = \sum\limits_{n=1}^d\sigma_n{(t)}f_n(\textbf{h}_{t}, \theta_t)
% \end{equation}
% with $\sigma_n{(t)} \in (0, 1)$.

% \subsection{Additional Background}

% \textbf{Riemannian Geometry and Properties of the Orthogonal Manifold}
% We provide here brief additional context regarding manifolds defined by orthogonality constraints. A \textit{Stiefel manifold} is given as: $\mathcal{ST}(d,k) = \{\mathbf{X} \in \mathbb{R}^{d \times k}\:\mathbf{X}^{\top}\mathbf{X}=\mathbf{I}_{k}\}$ for parameters $1 \leq k \leq d$. Thus the columns of $\mathbf{X} \in \mathcal{ST}(d,k)$ are conditioned to be orthogonal. In the special case when $k=d$ we obtain a manifold $\mathcal{O}(d)$ called the \textit{orthogonal group}. That manifold is conveniently equipped with group theory structure given by standard matrix multiplications (thus is an examples of the \textit{Lie group}), but, more importantly, is compact. Tangent spaces $\mathcal{T}_{\mathbf{X}}(\mathcal{O}(d))$ to $\mathcal{O}(d)$ in different $\mathbf{X} \in \mathcal{O}(d)$ are of the form $\{\mathbf{X}\Omega: \Omega \in \mathcal{AS}(d)\}$, where $\mathcal{AS}(d) = \{\Omega \in \mathbb{R}^{d \times d}: \Omega^{\top}=-\Omega\}$ is a set of antisymmetric matrices.  Thus $\mathcal{O}(d)$ is a ${d \choose 2}$-dimensional manifold. For our application, we use much lower-dimensional parameterizations that turn out to be very effective in practice. 

% \end{document}
